# Supplementary material for: Is Code Better Than Language for Algorithmic Reasoning
Source: arXiv:2606.15589 source file (2026-06-14)
Supplement: Supplementary file 1 [file complexity_stratified_route_accuracy.tex]

\subsection{Complexity-Stratified Route Accuracy}
\label{app:complexity_stratified_route_accuracy}

We stratify the main route-accuracy evaluation by the asymptotic complexity
class of each task. Across classes, Route~3 remains the main source of
improvement over Route~2, while Route~2 is close to Route~1.

\begin{center}
\footnotesize
\begin{tabular*}{\textwidth}{@{\extracolsep{\fill}}lrrrrrrrr@{}}
\toprule
Complexity & Tasks & Inst. & R1 & R2 & R3 & R2--R1 & $p_{2,1}$ & R3--R2 \\
\midrule
$O(1)$ & 3 & 180 & 46.2 & 47.3 & 86.2 & 1.0 & 0.0206 & 39.0 \\
$O(\log n)$ & 1 & 35 & 22.4 & 28.6 & 32.9 & 6.2 & 2.7e-04 & 4.3 \\
$O(n)$ & 4 & 135 & 4.8 & 5.0 & 7.5 & 0.2 & 0.635 & 2.5 \\
$O(n \log n)$ & 5 & 68 & 0.0 & 0.0 & 0.0 & 0.0 & 1 & 0.0 \\
$O(n^2)$ & 16 & 297 & 10.3 & 10.5 & 38.9 & 0.1 & 0.644 & 28.5 \\
$O(n^2 \log n)$ & 1 & 1 & 0.0 & 0.0 & 0.0 & 0.0 & 1 & 0.0 \\
$O(n^3)$ & 4 & 37 & 0.0 & 0.0 & 0.0 & 0.0 & 1 & 0.0 \\
NP-hard & 6 & 360 & 17.6 & 16.8 & 69.7 & -0.8 & 0.0278 & 53.0 \\
\bottomrule
\end{tabular*}
\captionof{table}{Route accuracy grouped by asymptotic complexity.}
\label{tab:appendix_complexity_routes}
\end{center}

\appendixresult{Accuracies and deltas in \cref{tab:appendix_complexity_routes} are percentages
or percentage points. McNemar tests are exact two-sided tests on paired outcomes.
The main route pattern is not an artifact of averaging together easy and hard
task families: the Route~3--Route~2 gain remains the largest observed change in
the high-support classes, while Route~2 stays close to Route~1.}

\paragraph{Task mapping.}
The 40-task analysis set is the broader 44-task route-analysis mapping after
excluding \texttt{segments\_intersect}, \texttt{knap}, \texttt{gcp}, and
\texttt{spp}. Within the retained set, the largest strata are $O(n^2)$
dynamic-programming, sorting, string, graph, and shortest-path tasks, plus
NP-hard ILP, edge-disjoint paths, shortest-path, and TSP tasks. Smaller strata
cover constant-time arithmetic, logarithmic binary search, linear
selection/string matching,
$O(n \log n)$ scheduling/sorting/hulls, $O(n^2 \log n)$ Kruskal MST, and cubic
dynamic-programming/shortest-path routines.
