# Supplementary material for: Is Code Better Than Language for Algorithmic Reasoning
Source: arXiv:2606.15589 source file (2026-06-14)
Supplement: Supplementary file 2 [file code_execution_failure_modes.tex]

\subsection{Code Execution Failure Modes}
\label{app:code_execution_failure_modes}

When Route~3 fails, failures are mostly semantic wrong answers rather than syntax or timeout failures. This supports the interpretation that code execution errors often originate in the generated program specification rather than in the Python runtime itself.

\begin{center}
\small
\begin{tabular}{lrrrr}
\toprule
Model & Wrong answer & Syntax error & Runtime error & Time limit \\
\midrule
Haiku & 56.26\% & 10.07\% & 1.88\% & 31.80\% \\
Codestral & 81.80\% & 5.87\% & 9.00\% & 3.33\% \\
Gemini 2.0 & 77.22\% & 14.65\% & 1.86\% & 6.27\% \\
Gemini 2.5 & 77.63\% & 17.10\% & 1.82\% & 3.45\% \\
GPT-4o mini & 72.93\% & 4.56\% & 18.97\% & 3.54\% \\
Mixtral & 60.67\% & 4.95\% & 32.14\% & 2.24\% \\
Total & 70.43\% & 9.34\% & 11.55\% & 8.67\% \\
\bottomrule
\end{tabular}
\captionof{table}{Distribution of Route~3 code-execution failures.}
\label{tab:appendix_code_failure_modes}
\end{center}

\appendixresult{\Cref{tab:appendix_code_failure_modes} is conditional on Route~3 failures and
excludes parse-only rows where execution completed but the returned value failed
parsing or type checks. This keeps the diagnostic focused on what happened after
code execution was actually attempted.}
