# Supplementary material for: Is Code Better Than Language for Algorithmic Reasoning
Source: arXiv:2606.15589 source file (2026-06-14)
Supplement: Supplementary file 3 [file coding_specialized_model_evaluation.tex]

\subsection{Coding-Specialized Model Evaluation}
\label{app:coding_specialized_model_evaluation}

We evaluate coding-specialized models to test whether models trained on code
show a different Route~2 pattern. Even for these models, replacing
natural-language traces with code traces changes little compared with replacing
LLM simulation by actual code execution.

\begin{center}
\footnotesize
\begin{tabular*}{0.92\textwidth}{@{\extracolsep{\fill}}lccc@{}}
\toprule
Model & NL & Sim & Code Exec \\
\midrule
x-ai/grok-code-fast-1 (25\% data) & 47.71\% (167/350) & 47.71\% (167/350) & 55.99\% (159/284) \\
qwen/qwen3-coder (25\% data) & 30.23\% (104/344) & 26.86\% (94/350) & 56.19\% (168/299) \\
codestral-2508 (original) & 19.89\% (943/4740) & 23.14\% (1097/4740) & 59.65\% (2266/3799) \\
\bottomrule
\end{tabular*}
\captionof{table}{Route accuracy for coding-specialized models. Each cell reports accuracy over correct / denominator.}
\label{tab:appendix_coding_models}
\end{center}

\appendixresult{Grok and Qwen use 25\% subset runs; Codestral uses the original evaluation run.
Rows use per-arm parse-normalized denominators: NL and Sim drop rows where
that arm failed to parse, while Code Exec keeps rows with successful code
execution. The 25\% subset rows broaden model coverage but are not pooled into
the main six-model estimate.}
