# Supplementary material for: Is Code Better Than Language for Algorithmic Reasoning
Source: arXiv:2606.15589 source file (2026-06-14)
Supplement: Supplementary file 4 [file frontier_model_sanity_checks.tex]

\subsection{Frontier Model Controlled-Subset Evaluation}
\label{app:frontier_model_sanity_checks}

We also evaluate two frontier models on a seed~1, 350-instance subset with
tool calling disabled and without patching or repair. These subset runs are not
used as the main estimate because the subset is smaller than the full six-model
evaluation, but they provide a controlled check that the route pattern is not
explained only by explicit tool calls.

\begin{center}
\small
\begin{tabular*}{\textwidth}{@{\extracolsep{\fill}}lrrr@{}}
\toprule
Model & Route 1 & Route 2 & Route 3 \\
\midrule
GPT-5.4 & 42.57\% (149/350) & 41.43\% (145/350) & 54.01\% (175/324) \\
Claude Opus 4.6 & 52.73\% (174/330) & 73.42\% (116/158) & 77.54\% (107/138) \\
\bottomrule
\end{tabular*}
\captionof{table}{Frontier tool-disabled controlled-subset route accuracy on the seed~1, 350-instance subset without patching or repair. Entries report accuracy with correct/denominator counts.}
\label{tab:appendix_frontier_nopatch}
\end{center}

\appendixresult{Reasoning-mode runs are excluded because hidden reasoning and
tool scaffolding confound the comparison; rows use seed~1, tool calling
disabled, and per-arm parse-normalized denominators.}
