# Supplementary material for: Is Code Better Than Language for Algorithmic Reasoning
Source: arXiv:2606.15589 source file (2026-06-14)
Supplement: Supplementary file 5 [file model_stratified_route_accuracy.tex]

\subsection{Model-Stratified Route Accuracy}
\label{app:model_stratified_route_accuracy}

We stratify the main route comparison by model to check whether the aggregate result is driven by one model family or scale regime. The Route~3 advantage persists across all six full-coverage models, while the Route~2--Route~1 difference is small and changes sign across models.

\begin{center}
\footnotesize
\setlength{\tabcolsep}{3pt}
\begin{tabular*}{\textwidth}{@{\extracolsep{\fill}}>{\raggedright\arraybackslash}p{0.35\textwidth}lrrrrrrrr@{}}
\toprule
Model & Type & Inst. & R1 & R2 & R3 & R2--R1 & $p_{2,1}$ & R3--R2 & $p_{3,2}$ \\
\midrule
anthropic/claude-haiku-4.5 & closed & 1113 & 23.3 & 23.6 & 47.1 & 0.3 & 0.612 & 23.5 & 2.4e-148 \\
google/gemini-2.0-flash-001 & closed & 1113 & 17.5 & 18.1 & 51.8 & 0.7 & 0.137 & 33.7 & 8.5e-298 \\
google/gemini-2.5-flash & closed & 1113 & 20.7 & 20.5 & 50.2 & -0.1 & 0.823 & 29.7 & 3.1e-238 \\
openai/gpt-4o-mini & closed & 1113 & 14.1 & 12.9 & 49.1 & -1.2 & 0.00663 & 36.1 & $<10^{-300}$ \\
mistralai/codestral-2508 & open & 1113 & 15.0 & 15.8 & 52.7 & 0.8 & 0.0279 & 36.9 & $<10^{-300}$ \\
mistralai/mixtral-8x22b-instruct & open & 1113 & 12.7 & 13.2 & 42.1 & 0.5 & 0.127 & 28.9 & 7.2e-253 \\
\bottomrule
\end{tabular*}
\captionof{table}{Route accuracy grouped by model.}
\label{tab:appendix_model_routes}
\end{center}

\appendixresult{Each row in \cref{tab:appendix_model_routes} has 1,113 unique problems and 3,339
paired route evaluations. Accuracies and deltas are percentages or percentage
points. This stratification shows that the execution gain is not an artifact of
mixing one weak or strong model into the aggregate.}
