# Supplementary material for: Is Code Better Than Language for Algorithmic Reasoning
Source: arXiv:2606.15589 source file (2026-06-14)
Supplement: Supplementary file 6 [file prompt_translation_shot_ablation.tex]

\subsection{Prompt Translation Shot Ablation}
\label{app:prompt_translation_shot_ablation}

The functional similarity test depends on translating code traces back into natural language. To test sensitivity to prompting, we vary the number of in-context examples used by the translator. More examples improve translated-trace utility and narrow the gap to native natural-language traces.

\begin{center}
\small
\begin{tabular*}{\textwidth}{@{\extracolsep{\fill}}lrrrrrr@{}}
\toprule
Shots & $x$ & $x$ + native NL & $x$ + translated NL & $\Delta$ native & $\Delta$ translated & Gap \\
\midrule
0 & 32.70\% & 55.70\% & 42.41\% & +23.00pp & +9.70pp & -13.29pp \\
1 & 32.70\% & 55.70\% & 45.78\% & +23.00pp & +13.08pp & -9.92pp \\
2 & 32.70\% & 55.70\% & 49.58\% & +23.00pp & +16.88pp & -6.12pp \\
3 & 32.70\% & 55.70\% & 48.52\% & +23.00pp & +15.82pp & -7.17pp \\
4 & 32.70\% & 55.70\% & 49.37\% & +23.00pp & +16.67pp & -6.33pp \\
5 & 32.70\% & 55.70\% & 50.00\% & +23.00pp & +17.30pp & -5.70pp \\
10 (reference) & 39.00\% & 56.50\% & 52.00\% & +17.50pp & +13.00pp & -4.50pp \\
\bottomrule
\end{tabular*}
\captionof{table}{Translation-additivity shot ablation for Claude Haiku 4.5.}
\label{tab:appendix_shot_ablation}
\end{center}

\appendixresult{Rows 0--5 in \cref{tab:appendix_shot_ablation} use a matched 25\% subset sweep.
The 10-shot reference row comes from the original main-evaluation setting and is
not from the same subset sweep. Here, $x$ is the question alone, $x$ + native NL
appends the original natural-language trace, and $x$ + translated NL appends the
natural-language trace translated from code.}
